# Supplementary material for: Clustering based on Random Graph Model embedding Vertex Features
Source: arXiv:0910.2107 source file (2009-10-12)
Supplement: Supplementary file 1 [file appendix.tex]

\appendix{Proof of the propositions}

\begin{proof}{Proof of the proposition \ref{ParameterEstimator}}

We have to maximize $E_{R(Z)}(J(\theta))$ with respect to each coefficient.

\begin{itemize}
\item{Estimation of $\pi_{ql}$}
\end{itemize}

We have, \[\frac{\partial E_{R(Z)}(J(\theta))}{\partial \pi_{ql}} = \displaystyle{\sum_ {\substack{i,j \\i \neq j}}}  R(Z_{iq})R(Z_{jl}) (\frac{x_{ij}}{\pi_{ql}} + \frac{-(1-x_{ij})}{1-\pi_{ql}})\]

Maximal value of $\pi_{ql}$ is obtained when the derivative is null,
$$
\frac{\partial E_{R(Z)}(J(\theta))}{\partial \pi_{ql}} = 0 \hspace{10pt} \Leftrightarrow \hspace{10pt} \displaystyle{\sum_ {\substack{i,j \\i \neq j}}}  R(Z_{iq})R(Z_{jl}) \pi_{ql} = \displaystyle{\sum_ {\substack{i,j \\i \neq j}}}  R(Z_{iq})R(Z_{jl}) x_{ij}
$$

So, the derivative is null iff,
$$
\hat{\pi}_{ql} = \frac{\displaystyle{\sum_ {\substack{i,j \\i \neq j}}}  R(Z_{iq})R(Z_{jl}) x_{ij}}{\displaystyle{\sum_ {\substack{i,j \\i \neq j}}}  R(Z_{iq})R(Z_{jl})}
$$

\begin{itemize}
\item{Estimation of $\alpha_q$}
\end{itemize}

In this case, we have to calculate the derivative under constraint. Indeed, $\displaystyle{\sum_{q}} \alpha_q$ needs to be equal to 1.

We have, $$\frac{\partial\left( E_{R(Z)}(J(\theta)) - \lambda(\displaystyle{\sum_{q}} \alpha_q - 1)\right)}{\partial \alpha_q} = \displaystyle{\sum_{i=1}^n } \frac{R(Z_{iq})}{\alpha_q} - \lambda$$

Where $\lambda$ is the Lagrange multiplier.
Maximal value of $\alpha_q$ is obtained when the derivative is null,
$$
\frac{\partial( E_{R(Z)}(J(\theta)) - \lambda(\displaystyle{\sum_{q}} \alpha_q - 1))}{\partial \alpha_q} = 0 \hspace{10pt} \Leftrightarrow  \hspace{10pt} \alpha_q = \displaystyle{\sum_{i=1}^n } \frac{R(Z_{iq})}{\lambda} 
$$

We know that $\displaystyle{\sum_{q}} \alpha_q$ = 1, so
$\displaystyle{\sum_{q=1}^Q} \displaystyle{\sum_{i=1}^n } \frac{R(Z_{iq})}{\lambda} =1$

Thus, $\lambda = \displaystyle{\sum_{q=1}^Q} \displaystyle{\sum_{i=1}^n } R(Z_{iq}) = n$ 

Thus, the estimated value of $\alpha_q$ is:
$$
\hat{\alpha}_q = \frac{\displaystyle{\sum_{i=1}^n}  R(Z_{iq})}{n}
$$

\begin{itemize}
\item{Estimation of $\mu_{ql}^{(1)}$}
\end{itemize}

In this case, we have to calculate the derivative of the normal distribution with respect to $\mu_{ql}^{(1)}$.

We have, $$\frac{\partial E_{R(Z)}(J(\theta))}{\partial \mu_{ql}^{(1)}} = \displaystyle{\sum_ {\substack{i,j \\i \neq j}}}  R(Z_{iq})R(Z_{jl})x_{ij}\frac{(-y_{ij} + \mu_{ql}^{(1)})}{2\sigma^2} $$

Maximal value of $\mu_{ql}^{(1)}$ is obtained when the derivative is null,
$$
\frac{\partial E_{R(Z)}(J(\theta))}{\partial \mu_{ql}^{(1)}} = 0 \hspace{10pt} \Leftrightarrow  \hspace{10pt} \displaystyle{\sum_ {\substack{i,j \\i \neq j}}}  R(Z_{iq})R(Z_{jl})x_{ij}\mu_{ql}^{(1)} = \displaystyle{\sum_ {\substack{i,j \\i \neq j}}}  R(Z_{iq})R(Z_{jl})y_{ij}x_{ij}
$$

Thus, the estimated value of  $\mu_{ql}^{(1)}$  is:
$$
\hat{\mu}_{ql}^{(1)} = \frac{\displaystyle{\sum_ {\substack{i,j \\i \neq j}}}  R(Z_{iq})R(Z_{jl}) x_{ij}y_{ij}}{\displaystyle{\sum_ {\substack{i,j\\i \neq j}}} R(Z_{iq})R(Z_{jl})x_{ij}}
$$

 $\mu_{ql}^{(2)}$ is obtained by the same method previously used.

\begin{itemize}
\item{Estimation of $\sigma^2$}
\end{itemize}

In this case, we have to calculate the derivative of the normal distribution with respect to $\sigma^2$.

We have, $$\frac{\partial E_{R(Z)}(J(\theta))}{\partial \sigma^2} = \displaystyle{\sum_ {\substack{i,j \\i \neq j}}}  R(Z_{iq})R(Z_{jl})\left[\frac{x_{ij}\left(-(y_{ij} - \hat{\mu}_{ql}^{(1)})^2+(y_{ij} - \hat{\mu}_{ql}^{(2)})^2\right) -(y_{ij} - \hat{\mu}_{ql}^{(2)})^2}{\sigma^4}+\frac{1}{2\sigma^2}\right] $$

Maximal value of $\sigma^2$ is obtained when the derivate is null,
$$
\frac{\partial E_{R(Z)}(J(\theta))}{\partial \sigma^2} = 0 \hspace{10pt} \Leftrightarrow  \\
$$
$$
 \displaystyle{\sum_ {\substack{i,j \\i \neq j}}}  R(Z_{iq})R(Z_{jl})\frac{x_{ij}\left((y_{ij} - \hat{\mu}_{ql}^{(1)})^2+(y_{ij} + \hat{\mu}_{ql}^{(2)})^2\right) -(y_{ij} + \hat{\mu}_{ql}^{(2)})^2}{\sigma^4} = \displaystyle{\sum_ {\substack{i,j \\i \neq j}}}  R(Z_{iq})R(Z_{jl})\frac{1}{\sigma^2}
$$

Thus, the estimated value of  $\sigma^2$  is:
$$
\hat{\sigma}^2 = \frac{\displaystyle{ \sum_ {\substack{i,j \\i \neq j}} \sum_{q,l}}  R(Z_{iq})R(Z_{jl}) \left[x_{ij}\left((y_{ij}-\hat{\mu}_{ql}^{(1)})^2-(y_{ij}-\hat{\mu}_{ql}^{(2)})^2\right) + (y_{ij}-\hat{\mu}_{ql}^{(2)})^2\right]}{\displaystyle{ \sum_ {\substack{i,j \\i \neq j}} \sum_{q,l}}  R(Z_{iq})R(Z_{jl})}
$$

\end{proof}

\begin{proof}{Proof of the proposition \ref{TauEstimator}}
\\
We have to maximize $E_{R(Z)}(J(\theta))$ with respect to the $\tau_{iq}$'s. Nonetheless, for all the nodes i, we must have $\sum_{q=1}^Q \tau_{iq}$ equal to 1.

So, we have to result the following equation:
$$
\forall i,q \hspace{10pt}  \frac{\partial\left( E_{R(Z)}(J(\theta)) - \displaystyle{\sum_{i=1}}\lambda_i(\displaystyle{\sum_{q}} \tau_{iq} - 1)))\right)}{\partial \tau_{iq}} = 0 \\
$$

With the constraint: $\forall i, \displaystyle{\sum_{q}} \tau_{iq} = 1  $

According to the expression of $E_{R(Z)}(J(\theta))$, we have,\\

\begin{eqnarray*}
\frac{\partial\left( E_{R(Z)}(J(\theta)) - \sum_{i=1}\lambda_i(\sum_{q} \tau_{iq} - 1)))\right)}{\partial \tau_{iq}} & = & \log(\alpha_q) + \sum_{j \neq i} \sum_{l}  \log\left( (\pi_{ql}^{x_{ij}} (1-\pi_{ql})^{1-x_{ij}})^{\tau_{jl}^{(m)}}\right)\\
&  & -log(\tau_{iq}) - 1 + \lambda_i \\
&  &- \frac{1}{2} \sum_{j \neq i} \sum_{l} \tau_{jl}\left(\frac{(y_{ij}-\mu_{ql})^2}{\sigma^2} + \log(2\pi\sigma^2)\right)
\end{eqnarray*}

This equation is equal to 0 and $\forall i, \displaystyle{\sum_{q}} \tau_{iq} = 1  $ iff $\hat{\tau}_{iq}$ satisfy the expected relation , $\exp(\lambda_i - 1)$ acts as a normalizing constant.

\end{proof}

\begin{proof}{Proof of the proposition \ref{ParameterEstimator2}}

Thanks to previous results, we have:

\begin{eqnarray*}
E_{R(Z)}(J(\theta)) & = & \displaystyle{\sum_{i=1}^n \sum_{q=1}^Q} R(z_{iq})\log(\alpha_q)\\ 
                    &   & +\displaystyle{\sum_ {\substack{i,j \\i \neq j}} \sum_{q,l}}  R(z_{iq})R(z_{jl}) (x_{ij}\log(\pi_{ql}) + (1-x_{ij})\log(1-\pi_{ql}))\\
		    &   &  +\displaystyle{\sum_ {\substack{i,j \\i \neq j}} \sum_{q,l}} R(z_{iq})R(z_{jl}) \left[ x_{ij}  \left(-\frac{(y_{ij} - \mu_{ql}^{(1)})^2}{2\sigma^2}  + \frac{(y_{ij} - \mu_{ql}^{(2)})^2}{2\sigma^2} \right) -  \frac{(y_{ij} - \mu_{ql}^{(2)})^2}{2\sigma^2}\right]\\
	       &   & +\displaystyle{\sum_ {\substack{i,j \\i \neq j}} \sum_{q,l}} R(z_{iq})R(z_{jl})\log( \frac{1}{\sqrt{2 \pi \sigma^2}})-\displaystyle{\sum_Z} R(Z)\log(R(Z))
\end{eqnarray*}

\begin{eqnarray*}
E_{Z|X,Y,\theta^{(m)}}(\log(P(X,Y,\theta)) & = & E_{Z|X,Y,\theta^{(m)}}(\log(P(X,Y,Z))|X,Y,\theta^{(m)})\\
&& - E_{Z|X,Y,\theta^{(m)}}(\log(P(Z|X,Y))|X,Y,\theta^{(m)})\\
& = & Q(\theta, \theta^{(m)}) - H(\theta, \theta^{(m)})
\end{eqnarray*}

With 
$$
H(\theta, \theta^{(m)}) = E_{Z|X,Y,\theta^{(m)}}(\log(P(Z|X,Y))|X,Y,\theta^{(m)}).
$$

To implement the estimation of the parameters, we first need to define the log-likelihood of the model. The equation \ref{Model:Dependency of $Y$ to $X$ and $Z$} allows to write this log-likelihood as follows:

\begin{eqnarray*}
\log(P(X,Y,Z)) = \log(P(Z))+ \log(P(X |Z))+ \log(P(Y | X,Z))
\end{eqnarray*}

\begin{eqnarray*}
P(Y | X,Z) & = & \prod_{i,j} P(Y_{ij} | X_{ij},Z_{i}) \\
& = & \prod_{i,j} \prod_{q,l} P(Y_{ij} | X_{ij},Z_{iq}Z_{jl}=1)^{z_{iq}z_{jl}}\\
& = & \prod_{i,j} \prod_{q,l} P(Y_{ij} | X_{ij},Z_{iq}Z_{jl}=1)^{x_{ij}Z_{iq}Z_{jl}} P(Y_{ij} | X_{ij},Z_{iq}Z_{jl}=1)^{(1-x_{ij})z_{iq}z_{jl}}
\end{eqnarray*}
Thus, 

\begin{eqnarray*}
\log(P(Y | X,Z)) & = &\sum_{i,j} \sum_{q,l} z_{iq}z_{jl}  x_{ij}\log(P(Y_{ij} | X_{ij},Z_{iq}Z_{jl}=1))\\
&  & + \sum_{i,j} \sum_{q,l} (1-x_{ij})\log(P(Y_{ij} | X_{ij},Z_{iq}Z_{jl}=1)) \\
& = & \displaystyle{\sum_ {\substack{i,j \\i \neq j}} \sum_{q,l}}  z_{iq}z_{jl}x_{ij}  (-\frac{(y_{ij} - \mu_{ql}^{(1)})^2}{2\sigma^2}  + \frac{(y_{ij} - \mu_{ql}^{(2)})^2}{2\sigma^2} ) -\displaystyle{\sum_ {\substack{i,j \\i \neq j}} \sum_{q,l}}  z_{iq}z_{jl}\frac{(y_{ij} - \mu_{ql}^{(2)})^2}{2\sigma^2}\\
	       &   & +\displaystyle{\sum_ {\substack{i,j \\i \neq j}} \sum_{q,l}} z_{iq}z_{jl}\log( \frac{1}{\sqrt{2 \pi \sigma^2}})
 \end{eqnarray*}

So, the complete log-likelihood is given by the following equation: 
\begin{eqnarray*}
\log(P(X,Y,Z)) & = & \displaystyle{\sum_{i=1}^n \sum_{q=1}^Q} z_{iq}\log(\alpha_q)+\displaystyle{\sum_ {\substack{i,j \\i \neq j}} \sum_{q,l}}  z_{iq}z_{jl} (x_{ij}\log(\pi_{ql}) + (1-x_{ij})\log(1-\pi_{ql}))\\
&   &  +\displaystyle{\sum_ {\substack{i,j \\i \neq j}} \sum_{q,l}}  z_{iq}z_{jl}x_{ij}  (-\frac{(y_{ij} - \mu_{ql}^{(1)})^2}{2\sigma^2}  + \frac{(y_{ij} - \mu_{ql}^{(2)})^2}{2\sigma^2} ) -\displaystyle{\sum_ {\substack{i,j \\i \neq j}} \sum_{q,l}}  z_{iq}z_{jl}\frac{(y_{ij} - \mu_{ql}^{(2)})^2}{2\sigma^2}\\
	       &   & +\displaystyle{\sum_ {\substack{i,j \\i \neq j}} \sum_{q,l}} z_{iq}z_{jl}\log( \frac{1}{\sqrt{2 \pi \sigma^2}})
\end{eqnarray*}
Where $\mu_{ql}^{(1)}$ and $\mu_{ql}^{(2)}$ are the parameters given in the previous part.\\

\end{proof}
